# Supplementary material for: Recognition of Heat-Induced Food State Changes by Time-Series Use of Vision-Language Model for Cooking Robot
Source: arXiv:2309.01528 source file (2023-09-06)
Supplement: Supplementary file 1 [file appendix.tex]

\section*{APPENDIX}

Appendixes should appear before the acknowledgment.
